# Supplementary material for: MatryoshkaKV: Adaptive KV Compression via Trainable Orthogonal Projection
Source: arXiv:2410.14731 source file (2025-05-16)
Supplement: Supplementary file 1 [file appendix_alg.tex]

\section{Search algorithm}
\label{appendix: search-algorithm}
Here we present our search algorithm.

\begin{algorithm}
\label{calculate-rate}
  \caption{Calculate Adaptive Compression Rate Of Each Head Inside LLM}
  \label{alg:rate}
  \SetKwInOut{KwIn}{Input}
  \SetKwInOut{KwOut}{Output}
  
  \KwIn{An LLM $ p \left( \boldsymbol{\cdot}\right)$ and an LLM equipped with low rank projections $ p' \left( \boldsymbol{\cdot}\right)$, a prompt $\vx$, compression rate interval $r$, target cache budget $\gamma$.}
  % \KwIn{Value truncate rate set $\mathcal{M}_V$, sorted in descending order}
  
  \KwOut{Two tensors $R^{K}$ and $R^{V}$ of shape $(\text{num-layer}, \text{num-head})$ specifying the key/value compression rates for each head in each layer.}

  \vspace{0.5cm}
  
  % \text{head-dim} $\gets$ \text{hidden-size} $\div$ \text{num-head} \\

   $R^{K} \gets \text{torch.full}(\text{head-dim}, (\text{num-layer}, \text{num-head}))$ \\

  $R^{V} \gets \text{torch.full}(\text{head-dim}, (\text{num-layer}, \text{num-head}))$ \\

  \vspace{0.5cm}
\Repeat{$\text{Budeget} \left( R^K, R^V \right) < \gamma$}{
    $\bigvarepsilon \gets \text{empty list}$ \\
    \For{$\text{Every Layer-}l$ $\text{in LLM}$  }{
        \For{$\text{Every Attention Head-}h$  }{
            $R^{K}_{l, h} \gets R^{K}_{l, h} - r$ \\
            
            $\epsilon_k \gets \displaystyle \KL \left( p \left( \boldsymbol{\cdot}  | \vx \right) \Vert  p' \left( \boldsymbol{\cdot}  | \vx; R^{K}, R^{V}  \right) \right)$ \\
            
            $\bigvarepsilon \gets [\bigvarepsilon, \epsilon_k] $  \\
            
            $R^{K}_{l, h} \gets R^{K}_{l, h} + r$ \\
            \vspace{0.5cm}
            
            $R^{V}_{l, h} \gets R^{V}_{l, h} - r$ \\
            
            $\epsilon_v \gets \displaystyle \KL \left( p \left( \boldsymbol{\cdot}  | \vx \right) \Vert  p' \left( \boldsymbol{\cdot}  | \vx; R^{K}, R^{V}  \right) \right)$ \\
            
            $\bigvarepsilon \gets [\bigvarepsilon, \epsilon_v] $  \\
            
            $R^{V}_{l, h} \gets R^{V}_{l, h} + r$ \\
        }
    }
    $R^K, R^V \gets \text{Update} \left( R^K, R^V, \bigvarepsilon \right)$ \\
  }
\end{algorithm}
